# Supplementary material for: Affordance Perception by a Knowledge-Guided Vision-Language Model with Efficient Error Correction
Source: arXiv:2407.13368 source file (2024-07-18)
Supplement: Supplementary file 1 [file appendix.tex]

\section{Appendix}\label{sec:appendix}

(ChatGPT example)

%\begin{figure}
%    \centering
%    \includegraphics[width=0.8\linewidth]{figures/ChatGPT_affordance_triplets.png}
%    \caption{Enter Caption}
%    \label{fig:enter-label}
%\end{figure}

\begin{figure}
    \centering
    \includegraphics[width=0.8\linewidth]{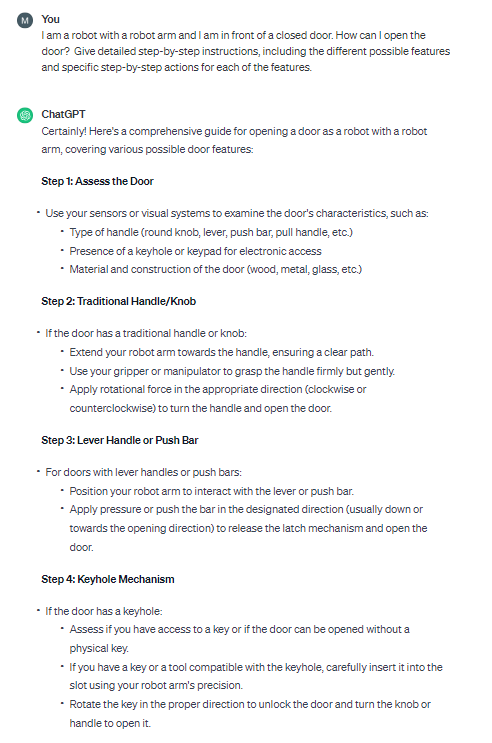}
    \caption{Enter Caption}
    \label{fig:enter-label}
\end{figure}

\begin{figure}
    \centering
    \includegraphics[width=0.8\linewidth]{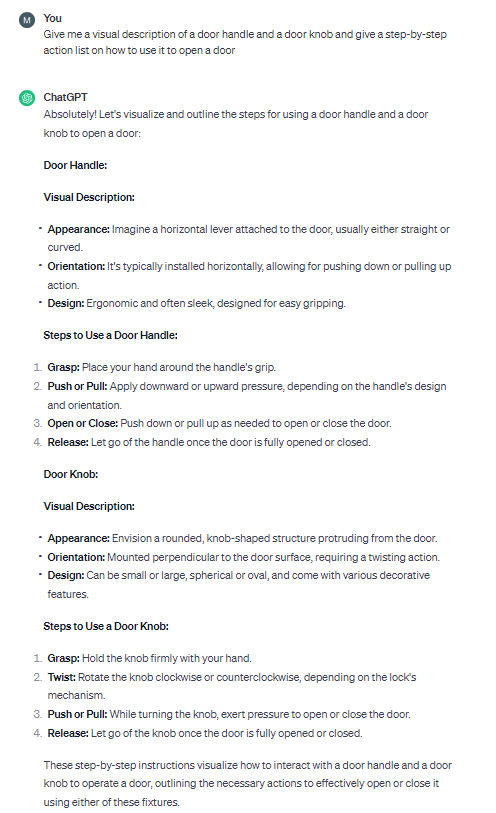}
    \caption{Enter Caption}
    \label{fig:enter-label}
\end{figure}
